# Supplementary material for: Robust Depth Enhancement via Polarization Prompt Fusion Tuning
Source: arXiv:2404.04318 source file (2024-04-05)
Supplement: Supplementary file 1 [file peft.tex]

\setlength{\belowcaptionskip}{-8pt}
\begin{figure}[!h]
  \centering
  
  \hspace{0.047\linewidth}
\begin{minipage}{0.168\linewidth}
\centering
    \small{GT depth}
\end{minipage}%
\hspace{0.001\linewidth}
\begin{minipage}{0.168\linewidth}
\centering
    \small{Sensor depth}
\end{minipage}%
\hspace{0.001\linewidth}
\begin{minipage}{0.168\linewidth}
\centering
    \small{\small{VPT \cite{jia2022visual}}}
\end{minipage}%
\hspace{0.001\linewidth}
\begin{minipage}{0.168\linewidth}
\centering
    \small{ViPT \cite{Zhu_2023_CVPR}}
\end{minipage}%
\hspace{0.001\linewidth}
\begin{minipage}{0.168\linewidth}
\centering
    \small{Ours (freezed)}
\end{minipage}\\[.8ex]
  
  \begin{minipage}{0.04\linewidth}
    \rotatebox{90}{\small{Active stereo}}
  \end{minipage}%
  \hspace{0.001\linewidth}
  \begin{minipage}{0.168\linewidth}
    \includegraphics[width=\linewidth]{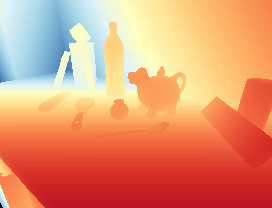}
  \end{minipage}%
  \hspace{0.001\linewidth}
  \begin{minipage}{0.168\linewidth}
    \includegraphics[width=\linewidth]{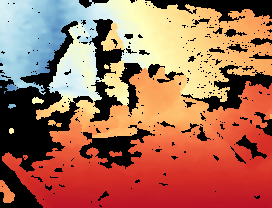}
  \end{minipage}%
  \hspace{0.001\linewidth}
  \begin{minipage}{0.168\linewidth}
    \includegraphics[width=\linewidth]{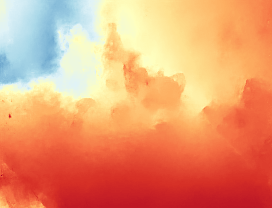}
  \end{minipage}%
  \hspace{0.001\linewidth}
  \begin{minipage}{0.168\linewidth}
    \includegraphics[width=\linewidth]{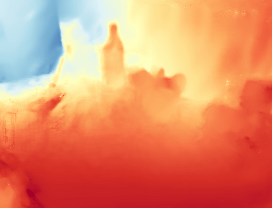}
  \end{minipage}%
  \hspace{0.001\linewidth}
  \begin{minipage}{0.168\linewidth}
    \includegraphics[width=\linewidth]{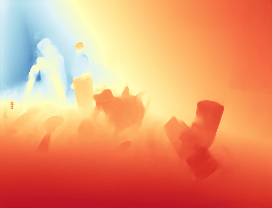}
  \end{minipage}\\[.5ex]

    \begin{minipage}{0.04\linewidth}
    \rotatebox{90}{\small{i-ToF}}
  \end{minipage}%
  \hspace{0.001\linewidth}
  \begin{minipage}{0.168\linewidth}
    \includegraphics[width=\linewidth]{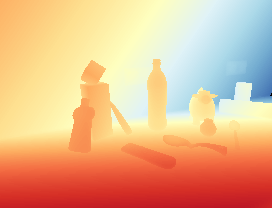}
  \end{minipage}%
  \hspace{0.001\linewidth}
  \begin{minipage}{0.168\linewidth}
    \includegraphics[width=\linewidth]{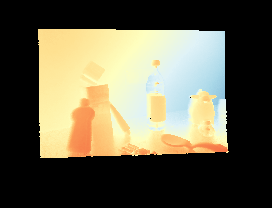}
  \end{minipage}%
  \hspace{0.001\linewidth}
  \begin{minipage}{0.168\linewidth}
    \includegraphics[width=\linewidth]{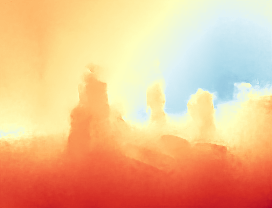}
  \end{minipage}%
  \hspace{0.001\linewidth}
  \begin{minipage}{0.168\linewidth}
    \includegraphics[width=\linewidth]{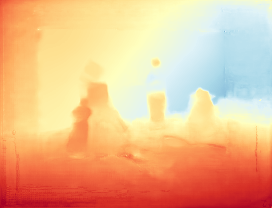}
  \end{minipage}%
  \hspace{0.001\linewidth}
  \begin{minipage}{0.168\linewidth}
    \includegraphics[width=\linewidth]{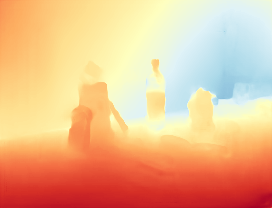}
  \end{minipage}\\[.5ex]

  \begin{minipage}{0.04\linewidth}
    \rotatebox{90}{d-ToF}
  \end{minipage}%
  \hspace{0.001\linewidth}
  \begin{minipage}{0.168\linewidth}
    \includegraphics[width=\linewidth]{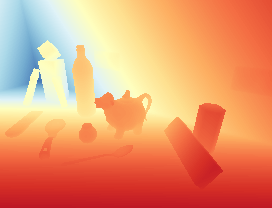}
  \end{minipage}%
  \hspace{0.001\linewidth}
  \begin{minipage}{0.168\linewidth}
    \includegraphics[width=\linewidth]{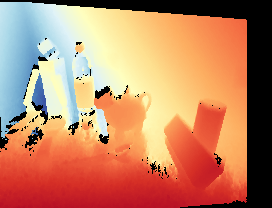}
  \end{minipage}%
  \hspace{0.001\linewidth}
  \begin{minipage}{0.168\linewidth}
    \includegraphics[width=\linewidth]{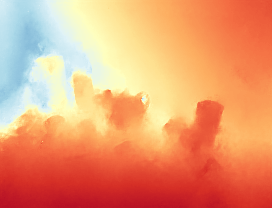}
  \end{minipage}%
  \hspace{0.001\linewidth}
  \begin{minipage}{0.168\linewidth}
    \includegraphics[width=\linewidth]{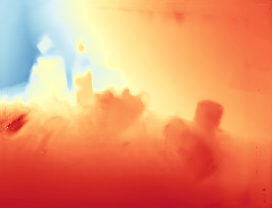}
  \end{minipage}%
  \hspace{0.001\linewidth}
  \begin{minipage}{0.168\linewidth}
    \includegraphics[width=\linewidth]{fig/Ablation-A/dtof/ours_freezed.png}
  \end{minipage}\\[.5ex]
  
  \caption{\textbf{Evaluation of Proposed Method as a Parameter-efficient Fine-tuning Method.} Our proposed method, with the pre-trained foundation model frozen during the training process, shows competitive performance on the dense geometry prediction problem studied.}
  \label{fig:peft}
\end{figure}
