# Supplementary material for: Robust Depth Enhancement via Polarization Prompt Fusion Tuning
Source: arXiv:2404.04318 source file (2024-04-05)
Supplement: Supplementary file 2 [file synth.tex]

\setlength{\belowcaptionskip}{-8pt}
\begin{figure}[!h]
  \centering
  
  \hspace{0.047\linewidth}
\begin{minipage}{0.149\linewidth}
\centering
    \small{GT depth}
\end{minipage}%
\hspace{0.001\linewidth}
\begin{minipage}{0.149\linewidth}
\centering
    \small{Sensor depth}
\end{minipage}%
\hspace{0.001\linewidth}
\begin{minipage}{0.149\linewidth}
\centering
    \small{DySPN~\cite{lin2022dynamic}}
\end{minipage}%
\hspace{0.001\linewidth}
\begin{minipage}{0.149\linewidth}
\centering
    \small{\cite{youmin2023completionformer}}
\end{minipage}%
\hspace{0.001\linewidth}
\begin{minipage}{0.149\linewidth}
\centering
    \small{\cite{youmin2023completionformer}$\dag$}
\end{minipage}%
\hspace{0.001\linewidth}
\begin{minipage}{0.149\linewidth}
\centering
    \small{Ours}
\end{minipage}\\[.8ex]
  
  \begin{minipage}{0.04\linewidth}
    \rotatebox{90}{\small{8 lines}}
  \end{minipage}%
  \hspace{0.001\linewidth}
  \begin{minipage}{0.149\linewidth}
    \includegraphics[width=\linewidth]{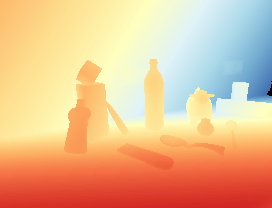}
  \end{minipage}%
  \hspace{0.001\linewidth}
  \begin{minipage}{0.149\linewidth}
    \includegraphics[width=\linewidth]{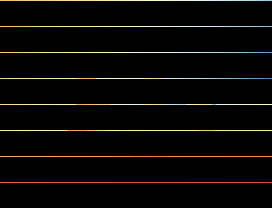}
  \end{minipage}%
  \hspace{0.001\linewidth}
  \begin{minipage}{0.149\linewidth}
    \includegraphics[width=\linewidth]{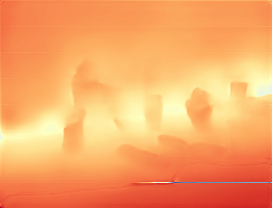}
  \end{minipage}%
  \hspace{0.001\linewidth}
  \begin{minipage}{0.149\linewidth}
    \includegraphics[width=\linewidth]{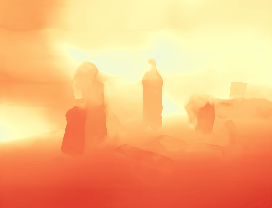}
  \end{minipage}%
  \hspace{0.001\linewidth}
  \begin{minipage}{0.149\linewidth}
    \includegraphics[width=\linewidth]{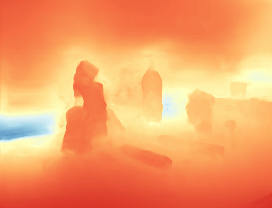}
  \end{minipage}%
  \hspace{0.001\linewidth}
  \begin{minipage}{0.149\linewidth}
    \includegraphics[width=\linewidth]{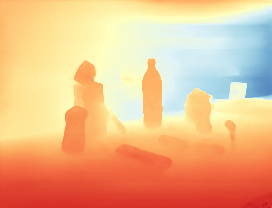}
  \end{minipage}\\[.5ex]

    \begin{minipage}{0.04\linewidth}
    \rotatebox{90}{\small{16 lines}}
  \end{minipage}%
  \hspace{0.001\linewidth}
  \begin{minipage}{0.149\linewidth}
    \includegraphics[width=\linewidth]{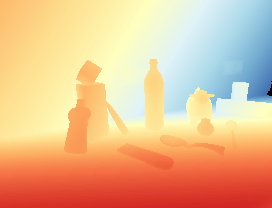}
  \end{minipage}%
  \hspace{0.001\linewidth}
  \begin{minipage}{0.149\linewidth}
    \includegraphics[width=\linewidth]{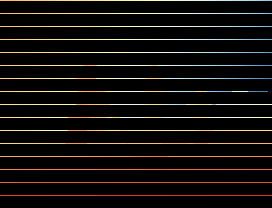}
  \end{minipage}%
  \hspace{0.001\linewidth}
  \begin{minipage}{0.149\linewidth}
    \includegraphics[width=\linewidth]{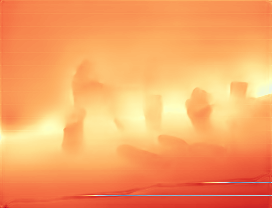}
  \end{minipage}%
  \hspace{0.001\linewidth}
  \begin{minipage}{0.149\linewidth}
    \includegraphics[width=\linewidth]{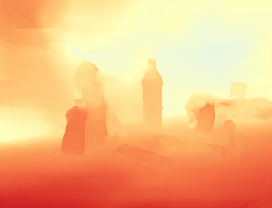}
  \end{minipage}%
  \hspace{0.001\linewidth}
  \begin{minipage}{0.149\linewidth}
    \includegraphics[width=\linewidth]{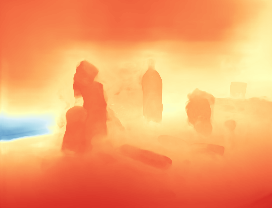}
  \end{minipage}%
  \hspace{0.001\linewidth}
  \begin{minipage}{0.149\linewidth}
    \includegraphics[width=\linewidth]{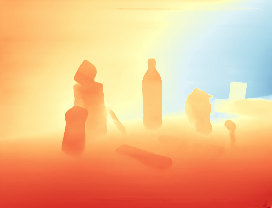}
  \end{minipage}\\[.5ex]
  
  \caption{\textbf{Evaluation of Proposed Method on Unseen Synthetic Data.} We simulate sparse measurement from typical LiDAR sensors by only keeping 8 and 16 scan lines of measurement. Our proposed method shows superior generalization ability to unseen depth degradation patterns. $\dag$ denotes that the model has been fine-tuned with pre-trained weights on a large-scale RGB-D dataset.}
  \label{fig:synth}
\end{figure}
