# Supplementary material for: Robust Depth Enhancement via Polarization Prompt Fusion Tuning
Source: arXiv:2404.04318 source file (2024-04-05)
Supplement: Supplementary file 3 [file architecture.tex]

\begin{table}[!ht]
    \footnotesize
	\begin{center}
        \resizebox{0.7\linewidth}{!}{
			\begin{tabular}{c|c|c|c}
				\toprule
				 Name & Backbone Layers & Fusion Layers & Output dimension \\

				 \midrule
				 
				 \multicolumn{4}{c}{\textbf{RGB and Depth Embedding}} \\
				 
				 \midrule
				 
				 input & --- & --- & $\begin{array}{c} \textrm{Polarization: }\; H \times W \times 7 \\ \textrm{RGB   Image: }\;\; H \times W \times 3 \\ \textrm{Sensor Depth: } H \times W \times 1 \end{array} $\\
     
				 \hline
				 conv\_separate & $ \begin{array}{c} \textrm{RGB: } \textrm{Conv} \; 3\times 3, 48  \\ \textrm{Sensor Depth: } \textrm{Conv} \; 3\times 3, 16 \end{array} $ & $ \begin{array}{c} \textrm{Polarization: } \textrm{Conv} \; 3\times 3, 48  \end{array} $ & $ \begin{array}{c} \textrm{Polarization Feature: } H \times W \times 48 \\ \textrm{RGB   Feature: } H \times W \times 48 \\ \textrm{Depth Feature: } H \times W \times 16  \end{array}$ \\
     
				 \hline
				conv1 &  $ \begin{array}{c} \textrm{concat [RGB}+ \textrm{Polarization,} \\ \textrm{ Depth Feature]} \\ \textrm{Conv} 3\times 3, 64   \end{array} $ & --- & $H \times W \times 64$ \\

				 \midrule
				 
				  \multicolumn{4}{c}{\textbf{Encoder}} \\
				 
				 \midrule
				 
				 conv2 & ResNet34~\cite{he2015deep} Block $\times 3$ & --- &$H \times W \times 64$ \\
				 \hline
				 
				conv3 & $\begin{array}{c} \textrm{ResNet34~\cite{he2015deep} Block} \times 4 \\ \textrm{PPFB (RGB, Polarization Feature)} \end{array}$ & $\begin{array}{c} \textrm{Conv} \; 3\times 3, \\ \textrm{stride}=2, \; 128  \\ \textrm{PPFB Block} \end{array}$ & $ \frac{1}{2}H\times \frac{1}{2}W \times 128$ \\
				 \hline
				 
				 conv4 & $\begin{array}{c} \textrm{IJCAT Blocks~\cite{youmin2023completionformer}} \\ \textrm{PPFB (RGB, Polarization Feature)} \end{array}$& $\begin{array}{c} \textrm{Conv} \; 3\times 3, \\ \textrm{stride}=2, \; 64  \\ \textrm{PPFB Block} \end{array}$ & $ \frac{1}{4}H\times \frac{1}{4}W \times 64$ \\ 
				 \hline
				conv5 & $\begin{array}{c} \textrm{IJCAT Blocks~\cite{youmin2023completionformer}} \\ \textrm{PPFB (RGB, Polarization Feature)} \end{array}$ & $\begin{array}{c} \textrm{Conv} \; 3\times 3, \\ \textrm{stride}=2, \; 128  \\ \textrm{PPFB Block} \end{array}$ & $ \frac{1}{8}H\times \frac{1}{8}W \times 128$ \\ 
				 \hline
				 conv6 & $\begin{array}{c}\textrm{IJCAT Blocks~\cite{youmin2023completionformer}} \\ \textrm{PPFB (RGB, Polarization Feature)} \end{array}$ & $\begin{array}{c} \textrm{Conv} \; 3\times 3, \\ \textrm{stride}=2, \; 320 \\ \textrm{PPFB Block} \end{array}$ & $ \frac{1}{16}H\times \frac{1}{16}W \times 320$ \\ 
				 \hline
				 conv7 & $\begin{array}{c}\textrm{IJCAT Blocks~\cite{youmin2023completionformer}}\\ \textrm{PPFB (RGB, Polarization Feature)} \end{array}$  & $\begin{array}{c} \textrm{Conv} \; 3\times 3, \\ \textrm{stride}=2, \; 512  \\ \textrm{PPFB Block} \end{array}$  & $ \frac{1}{32}H\times \frac{1}{32}W \times 512$ \\ 
				 
				 \midrule
				 \multicolumn{4}{c}{\textbf{Decoder}} \\
				 
				 \midrule
				 
				 dec6 & $ \begin{array}{c} 
				 \textrm{ConvTranspose}\; 3\times 3, \\ \textrm{stride}=2, \; 256 \\  \textrm{Convolutional Attention Layer} \\   
				 \end{array} $ & --- & $ \frac{1}{16}H\times \frac{1}{16}W \times 256 $ \\
				 
				 \hline
				 
				 dec5 & $ \begin{array}{c} 
				 \textrm{concat [dec6, conv6]} \\
				 \textrm{ConvTranspose}\; 3\times 3, \\ \textrm{stride}=2, \; 128 \\  \textrm{Convolutional Attention Layer} \\   
				 \end{array} $ & --- & $ \frac{1}{8}H\times \frac{1}{8}W \times 128 $ \\
				 
				 \hline
				 
				 dec4 & $ \begin{array}{c} 
				 \textrm{concat [dec5, conv5]} \\
				 \textrm{ConvTranspose}\; 3\times 3, \\ \textrm{stride}=2, \; 64 \\  \textrm{Convolutional Attention Layer} \\   
				 \end{array} $ & --- & $ \frac{1}{4}H\times \frac{1}{4}W \times 64 $ \\
				 
				 \hline
				 
				 dec3 & $ \begin{array}{c} 
				 \textrm{concat [dec4, conv4]} \\
				 \textrm{ConvTranspose}\; 3\times 3, \\ \textrm{stride}=2, \; 64 \\  \textrm{Convolutional Attention Layer} \\   
				 \end{array} $ & --- & $ \frac{1}{2}H\times \frac{1}{2}W \times 64 $ \\
				 
				 \hline
				 
				dec2 &  $ \begin{array}{c} 
				 \textrm{concat [dec3, conv3]} \\
				 \textrm{ConvTranspose}\; 3\times 3, \\ \textrm{stride}=2, \; 64 \\  \textrm{Convolutional Attention Layer} \\   
				 \end{array} $ & --- & $ H\times W \times 64 $ \\
				 
				 \midrule
				 
				 \multicolumn{4}{c}{\textbf{Initial Depth, Confidence, Non-local Neighbors, Affinity Prediction Head}} \\
				 
				 \midrule
				 
				 dec1 & $ \begin{array}{c} \textrm{concat [dec2, conv2]} \\  \textrm{Conv}\; 3\times 3, 64   \end{array}$  & --- & $H \times W \times 64$ \\ 
				 \hline
				 dec0 & $ \begin{array}{c} \textrm{concat [dec1, conv1]} \\  \textrm{Conv}\; 3\times 3, \eta   \end{array}$ & --- & $H \times W \times \eta$ \\
				 
				 \midrule
				 
				 \multicolumn{4}{c}{\textbf{SPN Refinement}} \\
				 
				 \midrule
				 
				 refine & $\begin{array}{c}\textrm{NLSPN~\cite{park2020non}}  \\ \textrm{with recurrent time} \; K=6 \end{array}$ & --- & $H \times W \times 1$ \\
				 
				 \bottomrule	
			\end{tabular}
		}
	\end{center}
	\caption{\textbf{Network Architecture Details of Proposed Polarization Prompt Fusion Tuning (PPFT) Method.} Here, `concat' denotes the concatenate operation along the channel dimension.}
	\label{tab: network parameters}
 \vspace{-0.3cm}
\end{table}
