# Supplementary material for: Robust Depth Enhancement via Polarization Prompt Fusion Tuning
Source: arXiv:2404.04318 source file (2024-04-05)
Supplement: Supplementary file 4 [file synthetic.tex]

\begin{table*}[!ht]
\footnotesize
\centering

\setlength{\belowcaptionskip}{-8pt}
\begin{tabular}{ >{\centering\arraybackslash}p{1.5cm} | p{4.3cm}  | >{\centering\arraybackslash}p{1.45cm} >{\centering\arraybackslash}p{1.4cm} >{\centering\arraybackslash}p{1.4cm} >{\centering\arraybackslash}p{1.4cm} >{\centering\arraybackslash}p{1.4cm}}
\toprule[1pt]

\multirow{2}{*}{$\begin{array}{cc} \text{Scanning}  \\ \text{Lines} 
\end{array}$ } & \multirow{2}{*}{Model} & RMSE (mm)$\downarrow$ & MAE (mm)$\downarrow$  & $\delta_1 \uparrow$ &$\delta_2 \uparrow $ & $\delta_3 \uparrow $\\
\hline

\multirow{4}{*}{8} 
& DySPN \cite{lin2022dynamic} & 225.00 & 166.13 & 0.518 & 0.776 & 0.909 \\

 & CompletionFormer \cite{youmin2023completionformer} & 109.60 & 78.94 & 0.855 & 0.990 & 0.995    \\

 & $\text{CompletionFormer}^\dag$~\cite{youmin2023completionformer} & 147.40  & 106.40 & 0.723 & 0.947 & 0.999   \\

 & Ours & \textbf{60.04} & \textbf{38.38} & \textbf{0.968} & \textbf{0.998} & \textbf{0.999}\\

\hline

\multirow{4}{*}{16} 
& DySPN \cite{lin2022dynamic} & 238.52 & 179.50 & 0.466 & 0.735 & 0.883\\

 & CompletionFormer \cite{youmin2023completionformer} & 93.00 & 67.56 & 0.907 & 0.995 & 0.999  \\
 
  & $\text{CompletionFormer}^\dag$~\cite{youmin2023completionformer} & 147.30 & 107.40 & 0.711 & 0.953 & 0.999  \\

  & Ours & \textbf{55.07} & \textbf{39.13} & \textbf{0.980} & \textbf{0.999} & \textbf{1.000}\\

\toprule[1pt]
\end{tabular}
\caption{\textbf{Quantitative Comparison on Synthetic LiDAR Depth Derived from the HAMMER~\cite{hammer} Dataset.} To compare, we select the best three models~\cite{lin2022dynamic,youmin2023completionformer} from the previous tested backbones. Our method obtains the best performance in both synthetic cases. $\dag$ denotes the model is fine-tuned with RGB images.}
\label{table:lidar}
\end{table*}
\setlength{\belowcaptionskip}{+8pt}
