# Supplementary material for: Robust Depth Enhancement via Polarization Prompt Fusion Tuning
Source: arXiv:2404.04318 source file (2024-04-05)
Supplement: Supplementary file 5 [file cross_modal_tl.tex]

\begin{table}[!t]
% \scriptsize
\footnotesize
\centering

\setlength{\belowcaptionskip}{-13pt}

\begin{tabular}{ p{1.0cm} | >{\centering\arraybackslash}p{0.6cm} >{\centering\arraybackslash}p{0.945cm} >{\centering\arraybackslash}p{0.48cm} >{\centering\arraybackslash}p{0.845cm} >{\centering\arraybackslash}p{2.01cm}}
\toprule[1pt]

  \multirow{2}{*}{Method} & RMSE & $\delta$RMSE & MAE & $\delta$MAE & Parameters \\

 & \multicolumn{4}{c}{(mm)$\downarrow$} & \\
 
\hline

 \cite{youmin2023completionformer}* & 313.60  & - & 241.40 & - & - \\

\hline

 \cite{youmin2023completionformer}$^\dag$ & 41.17  & - & 22.14 & - & 82.40M (100\%)\\
 
 VPT~\cite{jia2022visual} & 63.78  & +22.61 & 38.12  & +15.98 & 6.35M (7.7\%)\\

 ViPT~\cite{Zhu_2023_CVPR} & 52.30  & +11.13 & 30.39  & +8.25 & \textbf{2.15M (2.6\%)}\\
  
 $\text{Ours}^\ddagger$& \textbf{40.71}  & \textbf{-0.46} & \textbf{22.07} & \textbf{-0.07} & 7.32M (8.9\%)\\
 
\toprule[1pt]
\end{tabular}

\caption{\textbf{Ablation Experiments for Cross-modal Transfer Learning.} Parameters denote the number of trainable parameters, with the number in parenthesis indicating the proportion of the trainable parameters w.r.t. to all parameters. With our proposed Polarization Prompt Fusion Tuning (PPFT) the performance is improved significantly. * denotes that the foundation is pre-trained on the NYU-Depth V2 dataset~\cite{Silberman-ECCV12}. $\dag$ denotes that the model is trained from scratch with RGB images from the HAMMER dataset~\cite{hammer}, $\ddagger$ denotes that the foundation is freezed.}
\label{table:cross_modality}
\end{table}
